# Supplementary material for: Text-Conditioned Sampling Framework for Text-to-Image Generation with Masked Generative Models
Source: arXiv:2304.01515 source file (2023-04-04)

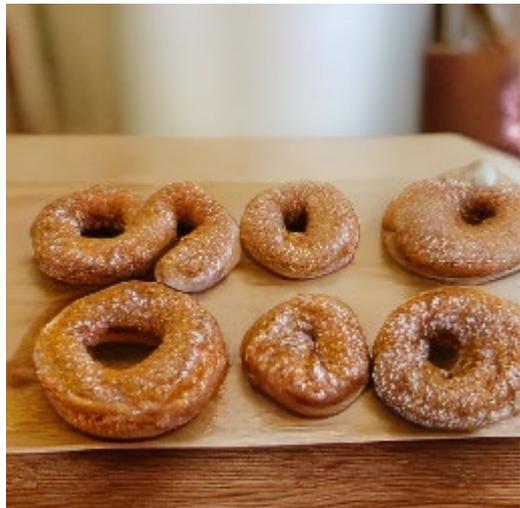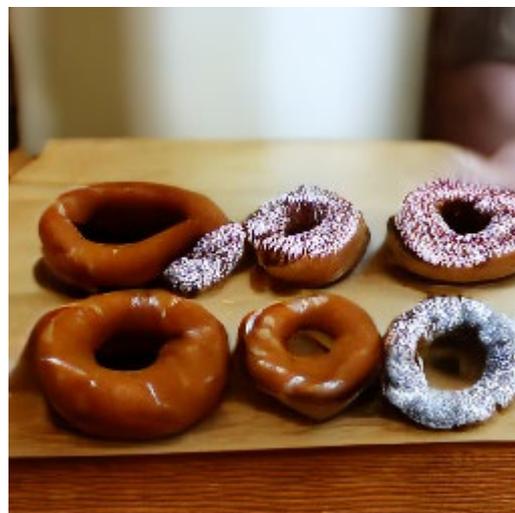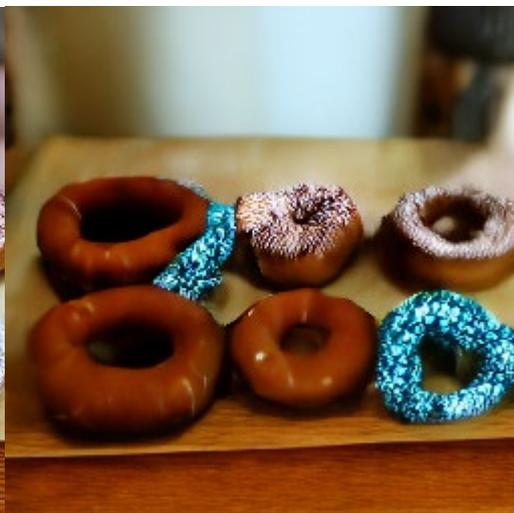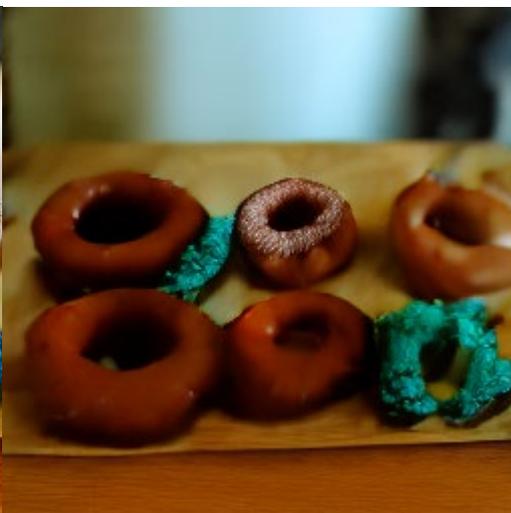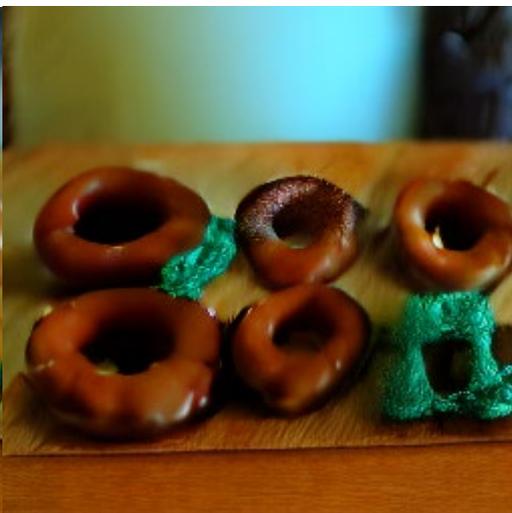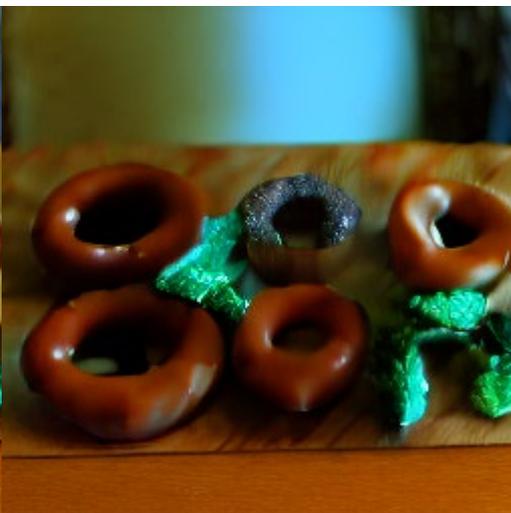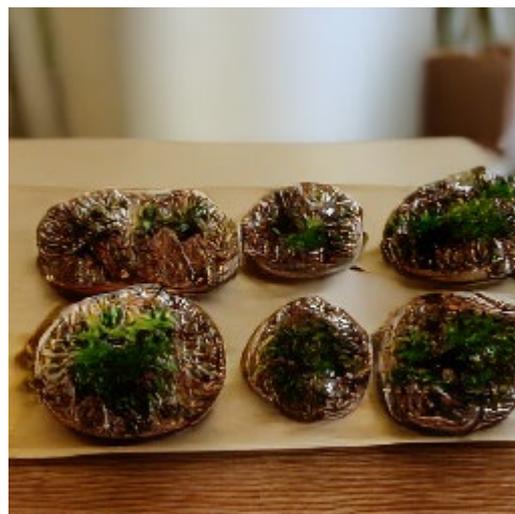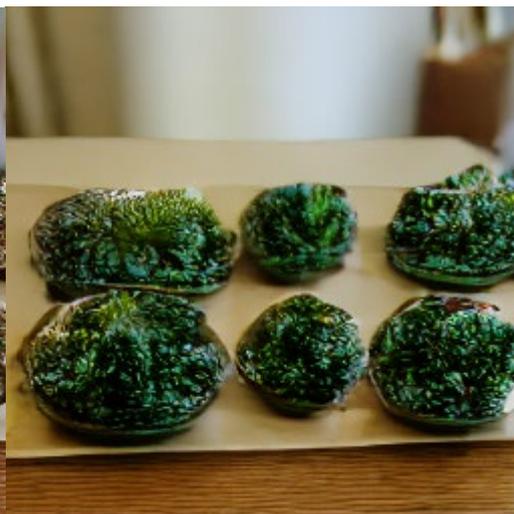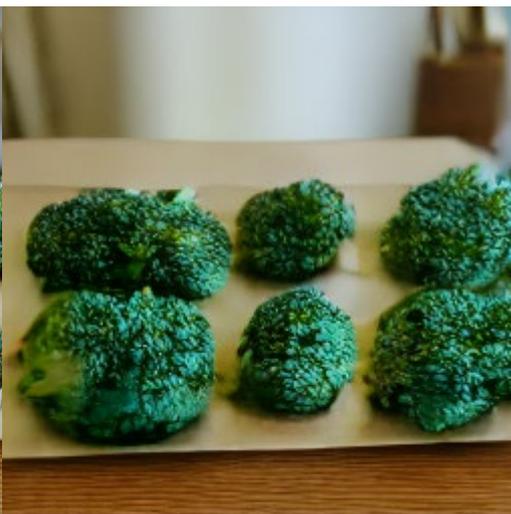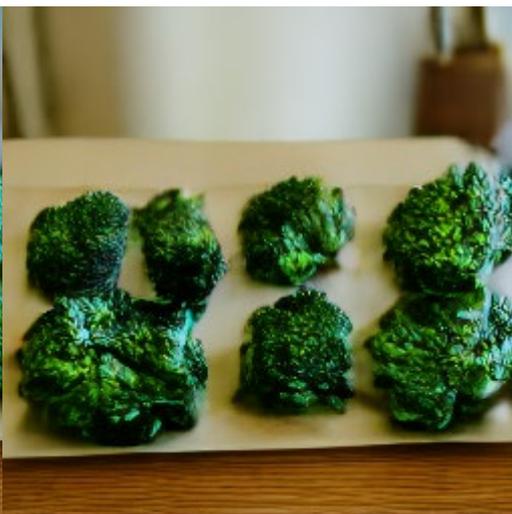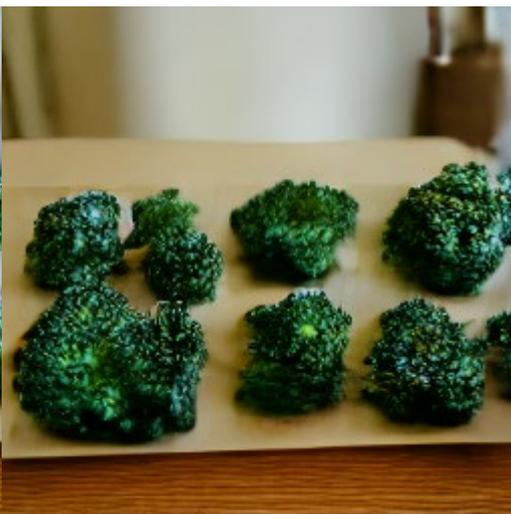

Supplement: Supplementary file 1 [file Appendix_mask_free.pdf]
